# Supplementary material for: Pseudo-chirality: a manifestation of Noether's theorem in non-Hermitian systems
Source: arXiv:2101.09239 source file (2021-01-22)
Supplement: Supplementary file 1 [file SM.pdf]

# Supplemental Material for “Pseudo-chirality: a manifestation of Noether’s theorem in non-Hermitian systems”

Jose D. H. Rivero and Li Ge

*Department of Physics and Astronomy, College of Staten Island, CUNY, Staten Island, NY 10314, USA and  
The Graduate Center, CUNY, New York, NY 10016, USA*

(Dated: July 28, 2020)

## CONTENTS

|                                                  |   |
|--------------------------------------------------|---|
| 1. Extended Ehrenfest’s theorem                  | 1 |
| 2. Definition of chiral symmetry                 | 1 |
| 3. Normalization of left and right eigenstates   | 2 |
| 4. Properties of pseudo-chirality                | 2 |
| 5. Wigner’s theorem                              | 2 |
| 6. Symmetries of the topological insulator laser | 3 |
| 7. Chiral edge states with disorder              | 4 |
| 8. Systems with asymmetric couplings             | 4 |
| 9. Application to Hermitian systems              | 5 |
| 10. Application to symmetric Hamiltonians        | 6 |
| References                                       | 7 |

## 1. EXTENDED EHRENFEST’S THEOREM

Using the unconjugated inner product defined by Eq. (4) in the main text, i.e.,

$$(\mu|\nu) \equiv \psi_\mu^T \psi_\nu, \quad (\text{S1})$$

we have shown the equation of motion for  $(A) \equiv (\psi|A|\psi)$  in Eq. (5) of the main text is

$$\frac{d}{dt}(A) = \frac{1}{i\hbar}(AH + H^T A) + \left(\frac{dA}{dt}\right). \quad (\text{S2})$$

This extended Ehrenfest’s theorem is derived similarly as the original one [1], as we show below. Using an overhead dot as the abbreviation for the time derivative, we find

$$\frac{d}{dt}(A) = (\psi|A|\dot{\psi}) + (\dot{\psi}|A|\psi) + (\psi|\dot{A}|\psi), \quad (\text{S3})$$

where the last term  $(\psi|\dot{A}|\psi) = (\dot{A})$  gives the second term in Eq. (S2) above. Next, we use the Schrödinger equation for  $\psi$  and its transpose, i.e.,

$$|\dot{\psi}\rangle = \frac{1}{i\hbar}H|\psi\rangle, \quad \langle\dot{\psi}| = \frac{1}{i\hbar}(\psi|H^T, \quad (\text{S4})$$

to simplify the other two terms in Eq. (S3):

$$\begin{aligned} (\psi|A|\dot{\psi}) + (\dot{\psi}|A|\psi) &= \frac{1}{i\hbar}[(\psi|AH|\psi) + (\psi|H^T A|\psi)] \\ &= \frac{1}{i\hbar}(AH + H^T A), \end{aligned}$$

which is the first term in Eq. (S2) above and Eq. (5) in the main text.

As we mentioned in the main text, the unconjugated inner product defined above is different from the biorthogonal product, specified by Eq. (8) in the main text. One could in principle introduce an alternative non-Hermitian expectation value using the biorthogonal product, which would require us to define a “left wave function”  $\bar{\psi}$  by

$$i\hbar\partial_t\bar{\psi}^T = \bar{\psi}^T H. \quad (\text{S5})$$

The matrix transpose is again included to make  $\bar{\psi}$  a column vector, similar to the definition of a left eigenstate. Now we can require the paired wave function  $\psi$  and left wave function  $\bar{\psi}$  to have the same expansion coefficients in the right and left eigenstate bases, i.e.,

$$\psi(t) = \sum_\mu a_\mu e^{-i\omega_\mu t} \psi_\mu, \quad \bar{\psi}(t) = \sum_\mu a_\mu e^{-i\omega_\mu t} \bar{\psi}_\mu, \quad (\text{S6})$$

and the alternative expectation value  $(A)_2$ , defined by  $\bar{\psi}^T A \psi$ , now satisfies

$$\frac{d}{dt}(A)_2 = \frac{1}{i\hbar}(AH + HA)_2 + \left(\frac{dA}{dt}\right)_2. \quad (\text{S7})$$

Therefore,  $(A)_2$  is a constant of motion when  $A$  is a chiral symmetry of the system, i.e.,  $\{A, H\} = AH + HA = 0$ .

## 2. DEFINITION OF CHIRAL SYMMETRY

The definition of chiral symmetry is unambiguous in (Hermitian) condensed matter systems [2], which is given by

$$\{\Xi, H\} = 0 \quad \text{or} \quad \Xi H \Xi^{-1} = -H \quad (\text{S8})$$

where  $\Xi$  is a linear operator. In the main text we have used the same definition in non-Hermitian systems, which was also the convention in several previous works on non-Hermitian symmetries [3–5]. Some authors [6, 7] recently introduced a different definition of chiral symmetry in non-Hermitian systems, using

$$\Xi H^\dagger \Xi^{-1} = -H \quad (\text{S9})$$

instead. To avoid any confusion, we suggest using the original definition of chiral symmetry also in non-Hermitian systems and referring to the symmetry defined by Eq. (S9) as pseudo-anti-Hermiticity, which had been introduced in Ref. [8] in 2002.

### 3. NORMALIZATION OF LEFT AND RIGHT EIGENSTATES

As we have noted in the main text, the left and right eigenstates of  $H$  are different in general when  $H$  is asymmetric, i.e.,  $H \neq H^T$ . The biorthogonal relation given by Eq. (8) in the main text then only specifies the scaling of the product  $\bar{\psi}_\mu^T \psi_\mu = 1$ : for two sets of  $\{\psi_\mu\}$  and  $\{\bar{\psi}_\mu\}$  that satisfy the biorthogonal relation, so do the following scaled sets:  $\psi'_\mu = r\psi_\mu$ ,  $\bar{\psi}'_\mu = \bar{\psi}_\mu/r$ . Therefore, if for the original sets we find  $A\psi_\mu = c\bar{\psi}_\nu$  when the system has pseudo-chirality, then we find  $A\psi'_\mu = c'\bar{\psi}'_\nu$  where  $c' = cr^2$ . In other words, we have the freedom to choose the constant  $c$ . Once  $c$  is chosen, the corresponding value  $c'$  in  $A\bar{\psi}'_\nu = c'\bar{\psi}_\mu$  is no longer arbitrary, as we have shown using Eq. (12) in the main text. Besides the example where  $A$  is anti-symmetric, another special case is when  $A$  is symmetric, leading to  $c = 1$  as in Fig. 1(d) for  $\Pi$  and Fig. 3(c) for  $A$  in the main text.

If the Hamiltonian is symmetric, then  $\bar{\psi}_\mu$  becomes the same as  $\psi_\mu$ , which indicates that  $\{\psi_\mu\}$  form an orthogonal basis by itself under the inner product defined in Eq. (S1), i.e.,  $(\mu|\nu) = 0$  ( $\mu \neq \nu$ ), due to the biorthogonal relation (8) in the main text. Caution should be exercised in the presence of an exceptional point, where some  $(\mu|\mu)$ 's become zero. Away from an exceptional point, the biorthogonal relation  $\psi_\mu^T \psi_\mu = (\mu|\mu) = 1$  then determines both the scaling and phase of  $\{\psi_\mu\}$ , leaving us with only a sign uncertainty. In the honeycomb lattice to be studied in Fig. S5, there are an odd number (i.e.,  $N = 13$ ) of states and a single zero mode.

### 4. PROPERTIES OF PSEUDO-CHIRALITY

In this section, we discuss a few important properties of pseudo-chirality. First, if we take the transpose of both sides of Eq. (6) in the main text, i.e.,

$$H = -[A^T]^{-1} H A^T \quad (\text{S10})$$

and then multiply  $A^T$  from the left and  $[A^T]^{-1}$  from the right, we find that  $A^T$  also leads to pseudo-chirality. However,  $A^T$  does not give rise to another constant of motion even when  $A$  is asymmetric. This is because

$$(A) = (A)^T = [\psi^T A \psi]^T = \psi^T A^T \psi = (A^T), \quad (\text{S11})$$

where the first equality holds because  $(A)$  is a number.

Similar to pseudo-Hermiticity, if  $G$  is another symmetry of the Hamiltonian satisfying  $[H, G] = 0$  or  $H = GHG^{-1}$ ,

then we find

$$H^T = -AHA^{-1} = -A[GHG^{-1}]A^{-1} = -[AG]H[AG]^{-1}.$$

In other words,  $AG$  is also a pseudo-chirality operator of  $H$ . The three  $\Pi_j$ 's to be discussed in Fig. S5 are examples of this observation, which are related by a CCW or CW rotation of  $120^\circ$ .

Related to the property above, we note that if two Hamiltonians are related by a similar transformation, i.e.,  $H_0 = GHG^{-1}$ , then if  $A_0$  is a pseudo-chirality operator of  $H_0$ , then  $A = G^T A_0 G$  is a pseudo-chirality operator of  $H$ . To prove it, we insert  $H_0 = GHG^{-1}$  into  $H_0^T = -A_0 H_0 A_0^{-1}$ :

$$[GHG^{-1}]^T = -A_0[GHG^{-1}]A_0^{-1} = -[A_0 G]H[A_0 G]^{-1}.$$

Its left-hand side is  $[G^T]^{-1} H^T G^T$ , and hence by multiplying  $G^T$  from the left and  $[G^T]^{-1}$  from the right, we find

$$H^T = -[G^T A_0 G]H[G^T A_0 G]^{-1}. \quad (\text{S12})$$

Therefore, we identify  $A = G^T A_0 G$  as a pseudo-chirality operator for  $H$ , indicating that  $(A) = (G^T A_0 G)$  is its constant of motion.

### 5. WIGNER'S THEOREM

Wigner's theorem is a fundamental proposition regarding possible forms of symmetries in quantum mechanics. It states that any symmetry transformation in the Hilbert space is represented by a linear (and unitary) or anti-linear (and anti-unitary) transformation of the Hilbert space. A linear symmetry transformation  $\mathcal{U}$  satisfies

$$\mathcal{U}(a\psi_1 + b\psi_2) = a\mathcal{U}\psi_1 + b\mathcal{U}\psi_2, \quad (\text{S13})$$

where  $\psi_{1,2}$  are two arbitrary quantum states and the complex numbers  $a, b$  are their linear superposition coefficients. In contrast, an anti-linear symmetry operator satisfies

$$\mathcal{U}(a\psi_1 + b\psi_2) = a^*\mathcal{U}\psi_1 + b^*\mathcal{U}\psi_2, \quad (\text{S14})$$

where the asterisk denotes the complex conjugation as usual.

Wigner's theorem is derived on the prerequisite that the transition probability  $|\langle\psi_1|\psi_2\rangle|^2$  is preserved after a symmetry transformation, which however does not apply in non-Hermitian systems. As a case in point, we consider the simple pseudo-spin Hamiltonian

$$H_s = \vec{b} \cdot \vec{\sigma} \quad (\text{S15})$$

discussed in the main text and the operator  $\Pi = b_2\sigma_1 - b_1\sigma_2$  that anticommutes with  $H_s$ , i.e.,

$$\{\Pi, H_s\} = b_1 b_2 \{\sigma_1, \sigma_1\} - b_2 b_1 \{\sigma_2, \sigma_2\} = 0. \quad (\text{S16})$$

Therefore, one inclines to define  $\Pi$  as a chiral symmetry of the system: it warrants that the spectrum of  $H_s$  is symmetric about the origin in the complex plane, i.e.,

$$\lambda_{1,2} = \pm \sqrt{b_1^2 + b_2^2 + b_3^2} \equiv \pm b_0, \quad (\text{S17})$$

and it transforms the two eigenstates of  $H_s$  into each other (up to a normalization constant):

$$\Pi\psi_1 = i(b_0 - b_3)\psi_2, \quad \psi_{1,2} = \begin{pmatrix} 1 \\ \frac{\pm b_0 - b_3}{b_1 - ib_2} \end{pmatrix}. \quad (\text{S18})$$

However, the quantity  $|\langle\psi_1|\psi_2\rangle|^2$  for two arbitrary states  $\psi_1 = [\psi_{11}, \psi_{21}]^T$  and  $\psi_2 = [\psi_{12}, \psi_{22}]^T$  is not preserved under this chiral symmetry:

$$\begin{aligned} \langle\Pi\psi_1|\Pi\psi_2\rangle &= (|b_1|^2 + |b_2|^2)\langle\psi_1|\psi_2\rangle \\ &\quad - 2i\text{Im}[b_1b_2^*](\psi_{11}^*\psi_{12} - \psi_{21}^*\psi_{22}). \end{aligned} \quad (\text{S19})$$

More specifically, there does not exist a universal scaling constant  $f$  (of  $\Pi$ ) that reduces the right hand side of this expression to  $\langle\psi_1|\psi_2\rangle$  times a phase factor, valid for all  $\psi_{1,2}$ .

This example illustrates the breakdown of the prerequisite of Wigner's theorem for a non-Hermitian Hamiltonian. We have also noted in the main text that the pseudo-spin Hamiltonian also has pseudo-chirality, given by  $A = \sigma_2$ :

$$AH + H^T A = b_2(\sigma_2^2 - \sigma_2^2) = 0. \quad (\text{S20})$$

Now if we consider  $|\langle\psi_1|\psi_2\rangle|^2$  again, it is in fact preserved under pseudo-chirality:

$$\langle A\psi_1|A\psi_2\rangle = \langle\psi_1|\psi_2\rangle. \quad (\text{S21})$$

Replacing the Hermitian inner product used above by the unconjugated inner product maintains these contrasting behaviors:

$$\begin{aligned} \langle\Pi\psi_1|\Pi\psi_2\rangle &= (b_2^2 - b_1^2)\langle\psi_1|\psi_2\rangle \\ &\quad + 2ib_1b_2(\psi_{11}\psi_{12} - \psi_{21}\psi_{22}), \end{aligned} \quad (\text{S22})$$

$$|\langle A\psi_1|A\psi_2\rangle|^2 = |\langle\psi_1|\psi_2\rangle|^2. \quad (\text{S23})$$

These observations indicate that many fundamental properties of non-Hermitian systems, including the inner products and their symmetries, still await further investigation.

## 6. SYMMETRIES OF THE TOPOLOGICAL INSULATOR LASER

The Hamiltonian of the  $n \times n$  topological lattice discussed in Figs. 2 and 3 in the main text is represented by a  $n^2 \times n^2$  matrix

$$\begin{aligned} H &= K + V = \begin{pmatrix} t_1 & t_2 & & \\ t_2^\dagger & t_1 & t_2 & \\ & & \ddots & t_2 \\ & & & t_2^\dagger & t_1 \end{pmatrix} + V \\ &= (\mathbb{1}_n \otimes t_1 + \xi_- \otimes t_2 + \xi_+ \otimes t_2^\dagger) + V. \end{aligned} \quad (\text{S24})$$

The potential energy term  $V$  is a diagonal matrix that captures the imaginary onsite detunings (i.e., gain and loss) and satisfies  $V = V^T = -V^\dagger$ . The kinetic energy term  $K$  includes the couplings in each column, i.e.,

$$t_1 \equiv g \begin{pmatrix} 0 & 1 & & \\ 1 & 0 & 1 & \\ & & \ddots & 1 \\ & & & 1 & 0 \end{pmatrix}, \quad (\text{S25})$$

as well as those between two neighboring columns, i.e.,

$$\xi_- \equiv \begin{pmatrix} 0 & 1 & & \\ & 0 & \ddots & \\ & & \ddots & 1 \\ & & & 0 \end{pmatrix}, \quad \xi_+ = \xi_-^\dagger, \quad (\text{S26})$$

with  $t_2 \equiv g \times \text{diag}(e^{i\pi/2}, e^{2i\pi/2}, \dots, e^{ni\pi/2})$ .  $t_{1,2}$  and  $\xi_\pm$  are  $n \times n$  matrices. The symbol “ $\otimes$ ” denotes the standard Kronecker product of matrices, and  $\mathbb{1}_n$  is a  $n \times n$  identity matrix.

Below we first prove that the system has pseudo-anti-hermiticity. As mentioned in the main text, the operator  $\eta$  is given by the sublattice operator  $C = P_A - P_B$ , which is a diagonal matrix and can be written as:

$$C = C_n \otimes C_n, \quad C_n = \text{diag}((-1)^0, \dots, (-1)^{n-1}).$$

The operator  $C$  acts on  $H^\dagger$  as follows:

$$\begin{aligned} CH^\dagger &= C_n \otimes C_n t_1^\dagger + C_n \xi_-^\dagger \otimes C_n t_2^\dagger + C_n \xi_+^\dagger \otimes C_n t_2 + CV^\dagger, \\ &= C_n \otimes C_n t_1 + C_n \xi_+ \otimes C_n t_2^\dagger + C_n \xi_- \otimes C_n t_2 - CV. \end{aligned}$$

Compare this expression to

$$\begin{aligned} HC &= C_n \otimes t_1 C_n + \xi_- C_n \otimes t_2 C_n + \xi_+ C_n \otimes t_2^\dagger C_n + VC \\ &= -C_n \otimes C_n t_1 - C_n \xi_- \otimes C_n t_2 - C_n \xi_+ \otimes C_n t_2^\dagger + CV \end{aligned}$$

and we find  $CH^\dagger = -CH$ , or equivalently,

$$CH^\dagger C^{-1} = -H, \quad (\text{S27})$$

where  $C^{-1} = C$ . Note that this proof of anti-pseudo-Hermiticity does not rely on the gain and loss landscape described by  $V$ . Therefore, anti-pseudo-Hermiticity is accountable for the symmetry protection of the topological insulator laser, where the pump-activated gain is only along the edge of the lattice. One example is given in Fig. 2(d) in the main text.

We have used  $C_n \xi_\pm = -\xi_\pm C_n$  to derive Eq. (S27), as well as  $C_n t_2 = t_2 C_n$ ,  $C_n t_2^\dagger = t_2^\dagger C_n$ , and  $CV = VC$  which hold because  $C_n$ ,  $t_2$ ,  $C$  and  $V$  are diagonal matrices.

Now if the system also has PT symmetry as shown in Fig. 2(a) in the main text, i.e.,  $[H, PT] = 0$ , where  $T$  is represented by the complex conjugation, then we find

$$H^T = [P^T]^{-1} H^\dagger P^T = -[P^T]^{-1} C^{-1} H C P^T. \quad (\text{S28})$$

In other words,  $H$  has pseudo-chirality with  $A = [CP^T]^{-1}$ . The parity operator  $P$  here takes the form

$$P \equiv P_n \otimes \mathbb{1}_n, \quad P_n \equiv \begin{pmatrix} & 1 \\ & \ddots \\ 1 & \end{pmatrix}, \quad (\text{S29})$$

and hence it satisfies  $P^T = P = P^{-1}$ . Therefore, we can write the pseudo-chirality operator as  $A = PC$  as given in the main text.

In order to prove that a disparity in the behavior of  $(A) = (\Psi|A|\Psi)$  emerges between  $n$  even or odd, according to the discussion in the main text, we only need to examine how  $A$  transforms under matrix transposition. In particular, we claimed that  $A^T = -A$  when  $n$  is even, and  $A^T = A$  when  $n$  is odd. First, we note that

$$PC = P_n C_n \otimes C_n, \quad (PC)^T = C_n P_n \otimes C_n. \quad (\text{S30})$$

Therefore, we only need to investigate the commutation relation between  $C_n$  and  $P_n$  for  $n$  even and odd. We define the following objects:

$$P_2 = \begin{pmatrix} & 1 \\ 1 & \end{pmatrix}, \quad C_2 = \begin{pmatrix} 1 & \\ & -1 \end{pmatrix},$$

$$P_3 = \begin{pmatrix} & 1 \\ & 1 \\ 1 & \end{pmatrix}, \quad C_3 = \begin{pmatrix} 1 & & \\ & -1 & \\ & & 1 \end{pmatrix}.$$

We observe that  $P_2 C_2 = -C_2 P_2$ , and that  $P_3 C_3 = C_3 P_3$ . We can construct recursively the  $C_n$ ,  $P_n$  matrices, for  $n > 3$ , by exploiting their block structure:

$$P_n = \begin{pmatrix} & 1 \\ & P_{n-2} \\ 1 & \end{pmatrix}, \quad C_n = \begin{pmatrix} 1 & & \\ & -C_{n-2} & \\ & & (-)^{n-1} \end{pmatrix},$$

such that

$$P_n C_n = \begin{pmatrix} & (-)^{n-1} \\ & -P_{n-2} C_{n-2} \\ 1 & \end{pmatrix},$$

$$C_n P_n = \begin{pmatrix} & 1 \\ (-)^{n-1} & -C_{n-2} P_{n-2} \end{pmatrix}.$$

We proceed by formal induction for  $n$  odd, by noting that if  $C_n P_n = P_n C_n$ , then

$$C_n P_n = \begin{pmatrix} & 1 \\ -P_{n-2} C_{n-2} & \end{pmatrix} = P_n C_n, \quad (\text{S31})$$

which proves that  $PC = (PC)^T$  for  $n$  odd. We use the same inductive tool to confirm that for  $n$  even, if  $C_{n-2} P_{n-2} = -P_{n-2} C_{n-2}$ , then  $C_n P_n = -P_n C_n$  as well, concluding that  $PC = -(PC)^T$  for  $n$  even.

## 7. CHIRAL EDGE STATES WITH DISORDER

To show that the chiral edge states studied in Fig. 3 of the main text, as well as the constant of motion ( $A$ ) due to pseudo-Hermiticity, are robust against symmetry-preserving disorder, we remove the lattice site at the center of the top row here. The energy eigenvalues of the system are shown in Fig. S1(a), which are symmetric about the real axis, imaginary axis, and the origin of the complex energy plane, reflecting its PT symmetry, pseudo-anti-Hermiticity, and pseudo-chirality, respectively. One representative chiral edge mode in the lower bandgap is highlighted by the large dot, and its wave function is shown in Fig. S1(b). Similar to its counterpart in the main text, this chiral edge mode transforms back into itself under a combined PT operation, and hence its energy is real. Fig. S1(d) shows a CW wave packet centered at the frequency of this mode, which is evolved in time to confirm the constant of motion given by ( $A$ ) [dashed line in Fig. S1(c)]. Since this wave packet consists of pure CW chiral edge modes, ( $A$ ) is zero as in Fig. 3 of the main text.

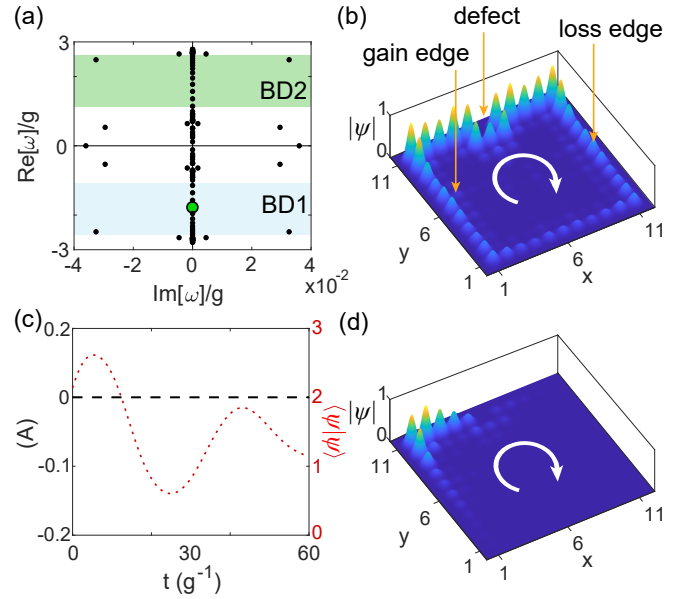

FIG. S1. Constants of motion due to pseudo-chirality in a topological non-Hermitian square lattice with a defect. The system is the same as that studied in Fig. 3 of the main text except for the defect. (a) Eigenvalues of the system. The large dot shows the chiral edge state plotted in (b). (c) Constant of motion ( $A$ ) for the pure CW chiral edge state in (d) (dashed line). The dotted line shows the non-conserved intensity that varies as a function of time.

## 8. SYSTEMS WITH ASYMMETRIC COUPLINGS

One particular application of Eq. (S12) is to find the resulting constant of motion in non-Hermitian systems

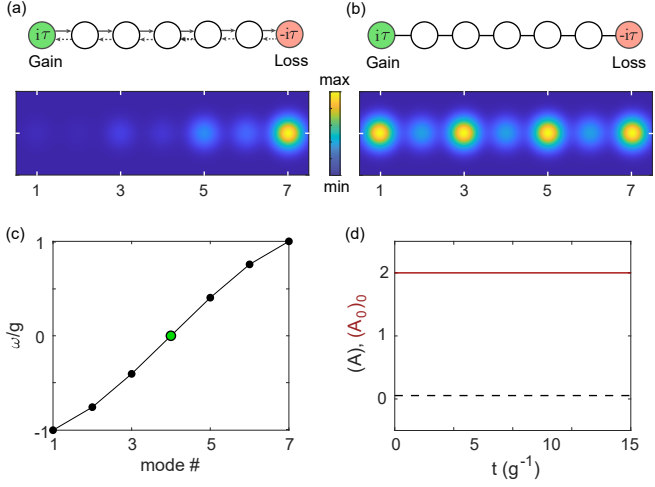

FIG. S2. Constants of motion due to pseudo-chirality in a non-Hermitian system with asymmetric couplings. (a,b) The schematics of this system and its equivalent lattice with symmetric couplings. The spatial profiles of their zero modes are also shown. (c) Identical energy spectrum of these two systems, with their zero modes marked by the large dot. (d) Constants of motion  $\langle A \rangle$  for  $H$  (dashed) and  $\langle A_0 \rangle_0$  for  $H_0$  (solid).

with asymmetric couplings [9, 10]. Here we take one example from Ref. [11] and study its constant of motion due to pseudo-chirality.

Consider the one dimensional lattice of  $N = 7$  sites in Fig. S2(a). The hopping to the left is denoted by  $t'$  (dashed arrow), and it is 30% of the hopping  $t$  to the right (solid arrow). Ref. [11] showed that its Hamiltonian  $H$  is transformed into another Hamiltonian  $H_0$  by  $H_0 = GHG^{-1}$ , where  $G$  is a diagonal matrix given by  $G = \text{diag}(1, s, s^2, \dots, s^{N-1})$  and  $s = \sqrt{t'/t}$ . This transformation leaves the on-site potentials unchanged, including the gain and loss at the two ends, and  $H_0$  has symmetric couplings given by  $\sqrt{tt'}$  [Fig. S2(b)].  $H$  and  $H_0$  have identical energy spectra as a result [Fig. S2(c)], including their zero (energy) modes (large dot). Here all energy eigenvalues are real because  $H_0$  is in its PT-symmetric phase with the gain and loss strength  $\tau$  equal to  $0.2t$ .

The corresponding wave functions of their zero modes are plotted in (a) and (b) respectively, showing a strongly localized mode  $\psi$  of  $H$  and a PT-symmetric zero mode [12]  $\tilde{\psi}$  of  $H_0$ . The localization of  $\psi$  is sometimes referred to as a non-Hermitian skin effect [9], and it can be understood from the transformation  $G$ :  $G$  is an imaginary gauge transformation between the two wave functions, i.e.,

$$\psi^{(n)} = \left[ \frac{1}{s} \right]^{n-1} \tilde{\psi}^{(n)} = e^{\frac{n-1}{2} \ln \frac{t}{t'}} \tilde{\psi}^{(n)}, \quad (\text{S32})$$

where the superscript  $n = 1, 2, \dots, N$  indicates the position along the lattice. For an extended  $\tilde{\psi}$ , we then find that  $\psi$  is localized on the right (left) of the system if  $t > t'$  ( $t < t'$ ).

Ref. [11] showed that both  $H$  and  $H_0$  have chiral symmetry, given by  $\Xi = GPCG^{-1}$  and  $A_0 = PC$  respectively. Here  $\mathcal{P}$  is the parity operator about the lattice center (i.e., the  $n = 4$  site), and  $C$  is the sublattice operator we have seen in the main text. Because only  $H_0$  is symmetric,  $A_0$  is a pseudo-chirality operator of  $H_0$  while  $\Xi$  does not make  $H$  pseudo-chiral. Nevertheless, Eq. (S12) tells us that  $A = G^T A_0 G = GPCG$  is indeed a pseudo-chirality operator of  $H$ , and we plot the resulting constant of motion  $\langle A \rangle$  in Fig. S2(d) together with  $\langle A_0 \rangle_0$  for  $H_0$ . Both quantities are for an initial wave function that has amplitude 1 at the two ends and zero elsewhere, and we see a big contrast between  $\langle A \rangle$  and  $\langle A_0 \rangle_0$ . To understand their difference, we note that  $\mathcal{PC}$  is an antidiagonal matrix with alternate elements of 1 and  $-1$ , and in this particular case  $\langle A_0 \rangle_0 = 2\tilde{\psi}^{(1)}\tilde{\psi}^{(N)} = 2$  while  $\langle A \rangle = 2\psi^{(1)}s^{N-1}\psi^{(N)} = 2s^{N-1} = 0.054$ . Therefore, their drastically different values for the same initial wave function are a direct reflection of the imaginary gauge transformation and how strong the non-Hermitian skin effect is.

## 9. APPLICATION TO HERMITIAN SYSTEMS

We also comment on the implication of pseudo-chirality in a Hermitian system. Since now  $H = H^\dagger$ , the definition of pseudo-chirality given by Eq. (6) in the main text has the same form as

$$\{H, A^{-1}\mathcal{K}\} = 0 \quad \text{or} \quad \{H, A^*\mathcal{K}\} = 0, \quad (\text{S33})$$

which can be interpreted as particle-hole symmetry. Here  $\mathcal{K}$  denotes the complex conjugation. Now let us express  $\langle A \rangle$  as

$$\langle A \rangle = \psi^T A \psi = [\psi^\dagger A^* \mathcal{K} \psi]^* = \langle A^* \mathcal{K} \rangle^*. \quad (\text{S34})$$

Because  $A^*\mathcal{K}$  is an anti-linear operator,  $\langle A^*\mathcal{K} \rangle$  [and hence  $\langle A \rangle$ ] is not an observable in the quantum mechanical sense and hence a hidden constant of motion. Nevertheless, we can construct analogous classical wave systems where the loss is negligible or inconsequential.  $\langle A \rangle$  can then be measured in principle, once a proper phase reference of the classical wave function is chosen.

For this purpose, we consider a Hamiltonian of the Bogoliubov-De Gennes form [13, 14]:

$$H_{\text{BdG}} = \begin{pmatrix} H & \Delta \\ -\Delta^* & -H^* \end{pmatrix}, \quad (\text{S35})$$

which originally describes a range of Bose-Einstein condensates with Cooper pairs including superconductivity.  $\Delta$  is an antisymmetric matrix while  $H$  is Hermitian to warranty the Hermiticity of  $H_{\text{BdG}}$ .  $H_{\text{BdG}}$  is a prime example of particle-hole symmetry, satisfying  $\{H_{\text{BdG}}, \sigma_x \mathcal{K}\} = 0$  where  $\sigma_x$  is the first Pauli matrix acting on the particle and hole blocks. From Eq. (S33) we know  $A = \sigma_x^* = \sigma_x$  gives rise to pseudo-chirality.

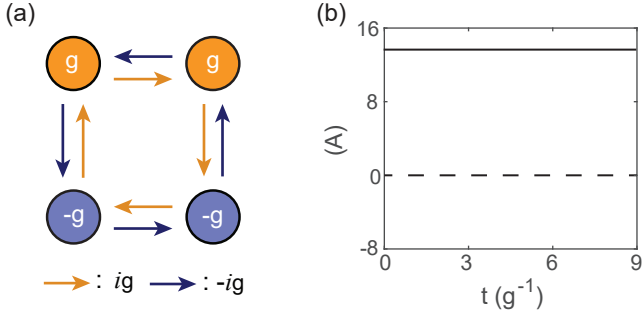

FIG. S3. “Hidden” constant of motion due to pseudo-chirality in a Hermitian system. (a) Schematic of the coupled optical elements. (b) Constants of motion with the two initial conditions specified in the text.

Now consider a simple case where  $h = (\mathbf{1}_2 + \sigma_y)g$  and  $\Delta = -\sigma_y g$ , where  $\mathbf{1}_2$  is the  $2 \times 2$  identity matrix and  $g$  is the amplitude of the couplings. This Hamiltonian can be constructed using four coupled optical cavities or waveguides, as we show schematically in Fig. S3(a). Now the pair excitation discussed in the main text can be demonstrated here as well. Most specifically, if an initial state is composed of only “particles” ( $\omega > 0$ ) i.e.,

$$\psi_1 = \frac{1}{\eta} \begin{pmatrix} u \\ -iu \\ 1 \\ -i \end{pmatrix}, \psi_2 = \frac{1}{\eta} \begin{pmatrix} u \\ iu \\ -1 \\ -i \end{pmatrix}, \quad (\text{S36})$$

or “holes” ( $\omega < 0$ ), i.e.,

$$\psi_3 = \frac{1}{\eta} \begin{pmatrix} -1 \\ i \\ u \\ -iu \end{pmatrix}, \psi_4 = \frac{1}{\eta} \begin{pmatrix} 1 \\ i \\ u \\ iu \end{pmatrix}, \quad (\text{S37})$$

the value of  $\langle A \rangle$  vanishes. Here  $u = 1 + \sqrt{2}$  and the normalization constant  $\eta = \sqrt{8 + 2\sqrt{2}}$ . If instead, the initial state is a mixture of particles and holes,  $\langle A \rangle$  is nonzero in general. These observations are shown in Fig. S3(b) with two initial conditions, one with only holes (dashed line;  $\psi = i\eta(\psi_3 - \psi_4)/2 = [-i, 0, 0, 1 + \sqrt{2}]^T$ ) and the other with two particles and two holes (solid line;  $\psi = i\eta(\psi_1 - \psi_2 + \psi_3 - \psi_4)/2 = [-i, 1 + \sqrt{2}, i, 1 + \sqrt{2}]^T$ ).

## 10. APPLICATION TO SYMMETRIC HAMILTONIANS

In the main text, we have briefly mentioned that the most studied form of a PT-symmetric Hamiltonian for a two-level system, i.e.,

$$H_{\text{PT}} = \begin{pmatrix} i\gamma & g \\ g & -i\gamma \end{pmatrix} = i\gamma\sigma_z + g\sigma_x, \quad (g, \gamma \in \mathbb{R}) \quad (\text{S38})$$

is a special case of the pseudo-spin Hamiltonian  $H_s$ . Since  $H_{\text{PT}}$  is symmetric, both  $\langle \sigma_y \rangle$  and  $\langle \Pi \rangle$  are constants of

motion, similar to what Fig. 1(d) in the main text shows and independent of whether the system is in the PT-symmetric or broken phase.

Here we also discuss its constant of motion due to pseudo-Hermiticity, following our discussion in Eq. (2) of the main text. Because  $H_{\text{PT}}$  is symmetric, it is also pseudo-Hermitian with  $A = \mathcal{P}^{-1} = \sigma_x$ . For an arbitrary state in this system, defined as  $\psi = [\psi_1, \psi_2]^T$ , we then find that

$$S_x \equiv \langle \sigma_x \rangle = \psi_1^* \psi_2 + \psi_1 \psi_2^* \quad (\text{S39})$$

is a constant of motion according to Eq. (2) in the main text. This conserved quantity was noted before [15, 16], but its physical understanding has been missing, especially in the PT-broken phase where  $\gamma > g$ : it is well known that the two eigenstates of  $H_{\text{PT}}$  in this regime are amplifying and decaying modes respectively, with eigenvalues  $\omega = \pm i\sqrt{\gamma^2 - g^2} \equiv i\omega_{\pm}$ . Therefore, one of them (the amplifying mode) quickly becomes dominant when  $t \gg \omega_{+}^{-1}$ , and both  $\psi_1$  and  $\psi_2$  diverge. Consequently, one would not have expected  $S_x$  to be a constant of motion, since it is proportional to the diverging quantity  $|\psi_1 \psi_2|$ . On the other hand, if one realizes that  $\psi_1$  and  $\psi_2$  are  $\pi/2$  out of phase in the amplifying mode, then one would expect the asymptotic value of  $S_z$  to be given by that of the amplifying mode, which is zero. The actual dynamics, however, maintains the initial value of  $S_z$ , which can be any finite complex number.

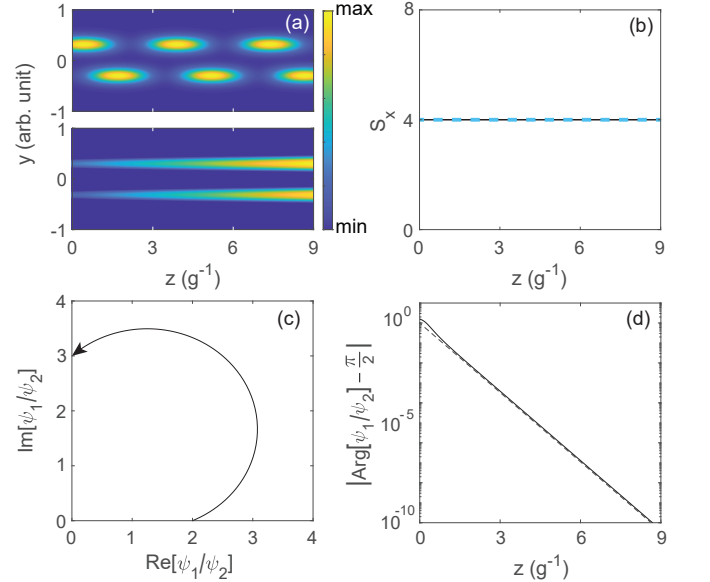

FIG. S4. Constant of motion in two coupled PT-symmetric waveguides along  $z$ . (a) Intensity evolution under the same initial condition in the PT-symmetric (upper; linear scale) and PT-broken (lower; logarithmic scale) phases. Transverse Gaussian mode profiles are imposed. (b)  $S_x$  in PT-symmetric (dashed) and PT-broken (solid) phases. (c,d) Evolution of the relative amplitude and phase in the two waveguides. Dashed line in (d) shows  $e^{-2\omega_{+}z} = e^{-8gz/3}$  as a comparison.  $\gamma = 0.4g, 5g/3$  are used in the two phases, respectively.

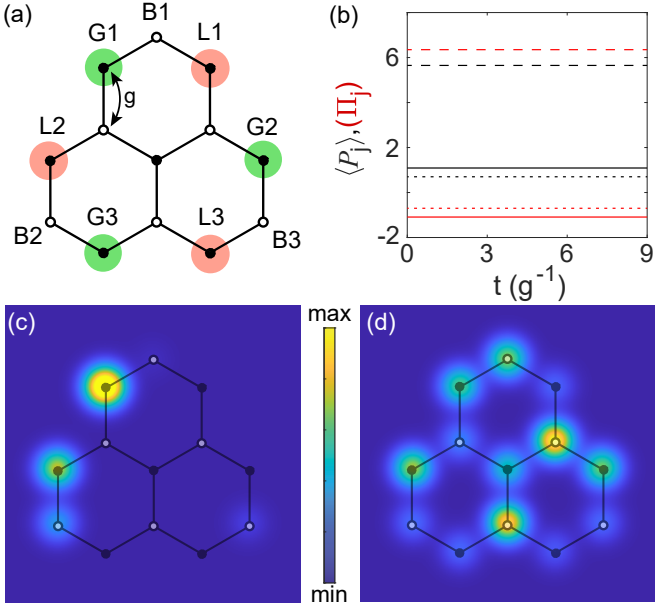

FIG. S5. Constants of motion in non-Hermitian tight-binding honeycomb lattice. (a) Schematic showing the gain ( $G_{1-3}$ ) and loss ( $L_{1-3}$ ) sites on the  $A$  sublattice and  $B_{1-3}$  on the  $B$  sublattice. (b) Constants of motion for the initial conditions  $\psi_{G1,B1,L2,B2,B3} = 2, 0.3, 1.5, -1, -0.5$  shown in (c), which evolves to the intensity pattern  $|\psi|^2$  in (d) at  $t = 1.6/g$ .

To illustrate this behavior, we use two coupled optical waveguides described by  $H_{PT}$  in the paraxial regime (Fig. S4), where the propagation direction  $z$  plays the role of time. The dynamical behaviors of this system are completely different in the PT-symmetric and PT-broken phases [17], one exhibiting power oscillations while the other showing an exponential growth [see Fig. S4(a)]. Nevertheless, they share the same constant of motion  $S_x$  [see Fig. S4(b)], set by their identical initial condition  $\psi_{1,2} = 2, 1$ . Fig. S4(c) further shows that the amplitude ratio of  $\psi_{1,2}$  does approach its value in the amplifying mode, which is  $3i$  in this case, but the value of  $S_x$  is still 0.6 instead of 0 given by the amplifying mode. This behavior is

made possible by an asymptote of  $\theta \equiv \text{Arg}[\psi_1/\psi_2] \rightarrow \pi/2$  [see Fig. S4(d)], with an exponent  $-2\omega_+ z$  to counter that in  $|\psi_1\psi_2| \sim e^{2\omega_+ z}$ :

$$S_x = 2|\psi_1\psi_2| \cos \theta \rightarrow 2|\psi_1\psi_2| \left( \frac{\pi}{2} - \theta \right). \quad (\text{S40})$$

We also consider a non-Hermitian tight-binding honeycomb lattice with three rings and the same nearest-neighbor coupling  $g \in \mathbb{R}$  everywhere [Fig. S5(a)]. It is PT-symmetric due to three pairs of symmetrically placed gain and loss of equal strength, i.e., with on-site imaginary potential  $\pm i\gamma$ . Here we take  $\gamma = 0.6g$  and all eigenvalues of  $H$  are real. The system can be described by the generalized dihedral group [18], and it has three different PT operators  $\mathcal{P}_j\mathcal{T}$  ( $j = 1, 2, 3$ ), with mirror reflections about the vertical,  $150^\circ$  ( $330^\circ$ ), and  $30^\circ$  ( $210^\circ$ ) axes, respectively. Because  $H$  is again symmetric and  $\mathcal{P}_j = \mathcal{P}_j^{-1}$ , the system is pseudo-Hermitian and  $\langle \mathcal{P}_j \rangle$ 's are constants of motion.  $\langle \mathcal{P}_j \rangle$ 's can still be interpreted as expectation or average values, and here all three of them are positive [Fig. S5(b)], indicating that the system hosts more PT-even eigenstates than PT-odd ones.

More important to our discussion, we note that the underlying Hermitian honeycomb lattice with real-valued couplings has sublattice symmetry, i.e.,  $\{H_0, C\} = 0$ , where  $C = P_A - P_B$  is the sublattice operator and  $P_{A,B}$  are the projection operators onto the two sublattices marked by open and closed dots in Fig. S5(a). NHPH symmetry then emerges automatically with the introduced gain and loss modulation [3], satisfying  $\{H, CT\} = 0$ . Together with the PT symmetries, they lead to three related non-Hermitian chiral symmetries [2, 11]:  $\Pi_j = \mathcal{P}_j(P_A - P_B)$ , with  $\Pi_{1,2,3} = \mathcal{R}_3\Pi_{3,1,2}$  where  $\mathcal{R}_3$  is a counterclockwise (CCW) rotation by  $120^\circ$ .

Recall that  $H$  is symmetric, and hence it also has pseudo-chirality that leads to three constants of motion, i.e.,  $\langle \Pi_j \rangle$ 's, using Noether's theorem indicated by Eq. (S2). Although  $\Pi_j$ 's are related by rotations, their "expectation values" are not as Fig. S5(b) (red lines) shows.

- [1] R. Shankar, *Principle of Quantum Mechanics*, 2nd ed. (Springer, New York, 1994).
- [2] M. Z. Hasan and C. L. Kane, Topological insulators, *Rev. Mod. Phys.* **82**, 3045 (2010).
- [3] L. Ge, Symmetry-protected zero-mode laser with a tunable spatial profile, *Phys. Rev. A* **95**, 023812 (2017).
- [4] B. Qi, L. Zhang, and L. Ge, Defect States Emerging from a Non-Hermitian Flatband of Photonic Zero Modes, *Phys. Rev. Lett.* **120**, 093901 (2018).
- [5] S. Malzard, C. Poli, and H. Schomerus, Topologically protected defect states in open photonic systems with non-Hermitian charge-conjugation and parity-time symmetry, *Phys. Rev. Lett.* **115**, 200402 (2015).
- [6] K. Kawabata, K. Shiozaki, M. Ueda, and M. Sato, Sym-

- metry and Topology in Non-Hermitian Physics, *Phys. Rev. X* **9**, 041015 (2019).
- [7] K. Kawabata, S. Higashikawa, Z. Gong, Y. Ashida, and M. Ueda, Topological unification of time-reversal and particle-hole symmetries in non-Hermitian physics, *Nature Commun.* **10**, 297 (2019).
- [8] G. Sclarici, Pseudoanti-Hermitian operators in quaternionic quantum mechanics. *J. Phys. A: Math. Gen.* **35**, 7493 (2002).
- [9] S. Weidemann, M. Kremer, T. Helbig, T. Hofmann, A. Stegmaier, M. Greiter, R. Thomale, and A. Szameit, Topological funneling of light, *Science* **368**, 311 (2020).
- [10] Z. Zhang et. al, Tunable topological charge vortex micro-laser, *Science* **368**, 760 (2020).

- [11] J. D. H. Rivero and L. Ge, Chiral symmetry in non-Hermitian systems: product rule and Clifford algebra, arXiv:1904.02231.
- [12] L. Ge, Parity-time symmetry in a flat-band system, Phys. Rev. A **92**, 052103 (2015).
- [13] N. N. Bogoliubov, J. Phys. (Moscow) **11**, 23 (1947).
- [14] P. G. de Gennes, *Superconductivity of Metals and Alloys* (Benjamin, New York, 1966).
- [15] M. Znojil, Conservation of pseudo-norm in PT symmetric quantum mechanics, Rendic. Circ. Mat. Palermo, Ser. II, Suppl. **72**, 211–218 (2004).
- [16] A. Mostafazadeh, Pseudo-Hermiticity versus PT symmetry: The necessary condition for the reality of the spectrum of a non-Hermitian Hamiltonian, J. Math. Phys. **43**, 205 (2002).
- [17] L. Feng, R. El-Ganainy, and L. Ge, Non-Hermitian photonics based on parity-time symmetry, Nat. Photon. **11**, 752–762 (2017).
- [18] L. Ge and A. D. Stone, Parity-Time Symmetry Breaking beyond One Dimension: The Role of Degeneracy, Phys. Rev. X **4**, 031011 (2014).
